# Supplementary material for: Exact Wave Packet Dynamics of Singlet Fission in Unsubstituted and Substituted Polyene Chains within Long-Range Interacting Models
Source: arXiv:1610.00562 ancillary file (2017-08-14)
Supplement: Supplementary file 1 [file supplemental_newest.pdf]

# Supplemental Material: Exact Wave Packet Dynamics of Singlet Fission in Unsubstituted and Substituted Polyene Chains within Long-Range Interacting Models

Suryoday Prodhan\* and S. Ramasesha†

*Solid State and Structural Chemistry Unit,  
Indian Institute of Science, Bangalore-560012, India.*

---

\* Electronic mail: [suryodayp@sscu.iisc.ernet.in](mailto:suryodayp@sscu.iisc.ernet.in)

† Electronic mail: [ramasesh@sscu.iisc.ernet.in](mailto:ramasesh@sscu.iisc.ernet.in)

The contents of this supplemental material are:

1. Properties of low-lying singlet states of butadiene dimer in the PPP model (Table. S1–S3).
2. Properties of low-lying singlet states of hexatriene dimer in the PPP model (Table. S4–S6).
3. Projection of  $1^1B \otimes 1^1A$  and  $T_1 \otimes T_1$  with eigenstates of the dimer system within Hückel model (Fig. S1).
4. Projection of  $1^1B \otimes 1^1A$  and  $T_1 \otimes T_1$  with eigenstates of the dimer system within Hubbard model (Fig. S2).
5. Time evolution profile of unsubstituted and substituted butadiene dimers (Fig. S3).
6. Time evolution profile of unsubstituted and substituted hexatriene dimers (Fig. S4).
7. Total yield and time evolution profile of unsubstituted and substituted butadiene, hexatriene and octatetraene dimers with  $|t_\perp| = X_\perp = 0.5$  eV in the PPP model (Fig. S5–S8).

TABLE S1. Properties of low-lying dimer eigenstates of substituted butadiene dimer ( $\epsilon = 1.0$ ).  $\langle \Psi | \Phi \rangle$  are projections of the dimer state on the direct product of the monomer states  $|\Phi\rangle$ , in the PPP model. The state  $|\Phi\rangle$  is a simple direct product of the states when the states on the two monomers are the same. For two different monomer states,  $|\phi\rangle$  and  $|\chi\rangle$ ,  $|\Phi\rangle = \frac{1}{\sqrt{2}}(|\phi\rangle_I \otimes |\chi\rangle_{II} + |\chi\rangle_I \otimes |\phi\rangle_{II})$ .  $d_I$  and  $d_{II}$  are average double occupancy per site within monomer I and II while  $s_I$  and  $s_{II}$  are the spin value of corresponding monomer units calculated from the spin-spin correlation functions.  $d_{I/II}^{(iso)}$  are the average double occupancies of isolated monomer eigenstates.  $\phi$ -s and  $\Psi$  are the eigenstates of the monomer and the dimer respectively.

| N | Orientation | $\Psi$ | $\phi_I$ | $\phi_{II}$ | $ \langle \Psi   \Phi \rangle $ | $d_I^{(iso)}$ | $d_{II}^{(iso)}$ | $d_I$ | $d_{II}$ | $s_I$ | $s_{II}$ |
|---|-------------|--------|----------|-------------|---------------------------------|---------------|------------------|-------|----------|-------|----------|
| 4 | V           | $S_0$  | $S_0$    | $S_0$       | 0.99                            | 0.18          | 0.18             | 0.18  | 0.18     | 0.004 | 0.004    |
|   |             | $S_1$  | $S_1$    | $S_0$       | 0.51                            | 0.13          | 0.18             | 0.19  | 0.19     | 0.49  | 0.49     |
|   |             |        | $S_2$    | $S_0$       | 0.48                            | 0.28          | 0.18             |       |          |       |          |
|   |             |        | $T_1$    | $T_1$       | 0.54                            | 0.12          | 0.12             |       |          |       |          |
|   |             | $S_2$  | $S_1$    | $S_0$       | 0.93                            | 0.13          | 0.18             | 0.15  | 0.15     | 0.06  | 0.06     |
|   |             |        | $S_2$    | $S_0$       | 0.20                            | 0.28          | 0.18             |       |          |       |          |
|   |             | $S_3$  | $S_2$    | $S_0$       | 0.68                            | 0.28          | 0.18             | 0.18  | 0.18     | 0.58  | 0.58     |
|   |             |        | $T_1$    | $T_1$       | 0.64                            | 0.12          | 0.12             |       |          |       |          |
|   |             | $S_4$  | $S_1$    | $S_0$       | 0.82                            | 0.13          | 0.18             | 0.14  | 0.14     | 0.32  | 0.32     |
|   |             |        | $S_2$    | $S_0$       | 0.32                            | 0.28          | 0.18             |       |          |       |          |
|   |             |        | $T_1$    | $T_1$       | 0.46                            | 0.12          | 0.12             |       |          |       |          |
|   |             | $S_5$  | $S_1$    | $S_0$       | 0.23                            | 0.13          | 0.18             | 0.24  | 0.24     | 0.04  | 0.04     |
|   |             |        | $S_2$    | $S_0$       | 0.95                            | 0.28          | 0.18             |       |          |       |          |
|   | H           | $S_0$  | $S_0$    | $S_0$       | 0.99                            | 0.18          | 0.18             | 0.18  | 0.18     | 0.003 | 0.003    |
|   |             | $S_1$  | $S_1$    | $S_0$       | 0.82                            | 0.13          | 0.18             | 0.20  | 0.20     | 0.16  | 0.16     |
|   |             |        | $S_2$    | $S_0$       | 0.47                            | 0.28          | 0.18             |       |          |       |          |
|   |             |        | $T_1$    | $T_1$       | 0.28                            | 0.12          | 0.12             |       |          |       |          |
|   |             | $S_2$  | $S_1$    | $S_0$       | 0.99                            | 0.13          | 0.18             | 0.15  | 0.15     | 0.01  | 0.01     |
|   |             | $S_3$  | $S_1$    | $S_0$       | 0.30                            | 0.13          | 0.18             | 0.12  | 0.12     | 0.93  | 0.93     |
|   |             |        | $T_1$    | $T_1$       | 0.95                            | 0.12          | 0.12             |       |          |       |          |
|   |             | $S_4$  | $S_1$    | $S_0$       | 0.48                            | 0.13          | 0.18             | 0.19  | 0.19     | 0.03  | 0.03     |
|   |             |        | $S_2$    | $S_0$       | 0.86                            | 0.28          | 0.18             |       |          |       |          |
|   |             | $S_5$  | $S_2$    | $S_0$       | 0.98                            | 0.28          | 0.18             | 0.23  | 0.23     | 0.03  | 0.03     |

TABLE S2. Properties of low-lying dimer eigenstates of substituted butadiene dimer ( $\epsilon = 2.0$ ).  $\langle \Psi | \Phi \rangle$  are projections of the dimer state on the direct product of the monomer states  $|\Phi\rangle$ , in the PPP model. The state  $|\Phi\rangle$  is a simple direct product of the states when the states on the two monomers are the same. For two different monomer states,  $|\phi\rangle$  and  $|\chi\rangle$ ,  $|\Phi\rangle = \frac{1}{\sqrt{2}}(|\phi\rangle_I \otimes |\chi\rangle_{II} + |\chi\rangle_I \otimes |\phi\rangle_{II})$ .  $d_I$  and  $d_{II}$  are average double occupancy per site within monomer I and II while  $s_I$  and  $s_{II}$  are the spin value of corresponding monomer units calculated from the spin-spin correlation functions.  $d_{I/II}^{(iso)}$  are the average double occupancies of isolated monomer eigenstates.  $\phi$ -s and  $\Psi$  are the eigenstates of the monomer and the dimer respectively.

| N | Orientation | $\Psi$ | $\phi_I$ | $\phi_{II}$ | $ \langle \Psi   \Phi \rangle $ | $d_I^{(iso)}$ | $d_{II}^{(iso)}$ | $d_I$ | $d_{II}$ | $s_I$ | $s_{II}$ |
|---|-------------|--------|----------|-------------|---------------------------------|---------------|------------------|-------|----------|-------|----------|
| 4 | V           | $S_0$  | $S_0$    | $S_0$       | 0.99                            | 0.20          | 0.20             | 0.20  | 0.20     | 0.005 | 0.005    |
|   |             | $S_1$  | $S_1$    | $S_0$       | 0.79                            | 0.26          | 0.20             | 0.22  | 0.22     | 0.30  | 0.30     |
|   |             |        | $T_1$    | $T_1$       | 0.33                            | 0.12          | 0.12             |       |          |       |          |
|   |             | $S_2$  | $S_1$    | $S_0$       | 0.86                            | 0.26          | 0.20             | 0.20  | 0.20     | 0.04  | 0.04     |
|   |             |        | $S_2$    | $S_0$       | 0.45                            | 0.13          | 0.20             |       |          |       |          |
|   |             | $S_3$  | $S_1$    | $S_0$       | 0.45                            | 0.26          | 0.20             | 0.21  | 0.21     | 0.05  | 0.05     |
|   |             |        | $S_2$    | $S_0$       | 0.83                            | 0.13          | 0.20             |       |          |       |          |
|   |             | $S_4$  | $S_1$    | $S_0$       | 0.25                            | 0.26          | 0.20             | 0.16  | 0.16     | 0.63  | 0.63     |
|   |             |        | $T_1$    | $T_1$       | 0.70                            | 0.12          | 0.12             |       |          |       |          |
|   |             | $S_5$  | $S_2$    | $S_0$       | 0.35                            | 0.13          | 0.20             | 0.15  | 0.15     | 0.42  | 0.42     |
|   |             |        | $T_1$    | $T_1$       | 0.54                            | 0.12          | 0.12             |       |          |       |          |
|   |             |        |          |             |                                 |               |                  |       |          |       |          |
|   |             |        |          |             |                                 |               |                  |       |          |       |          |
|   |             |        |          |             |                                 |               |                  |       |          |       |          |
|   | H           | $S_0$  | $S_0$    | $S_0$       | 0.99                            | 0.20          | 0.20             | 0.20  | 0.20     | 0.003 | 0.003    |
|   |             | $S_1$  | $S_1$    | $S_0$       | 0.96                            | 0.26          | 0.20             | 0.24  | 0.24     | 0.04  | 0.04     |
|   |             |        | $S_2$    | $S_0$       | 0.15                            | 0.13          | 0.20             |       |          |       |          |
|   |             | $S_2$  | $S_1$    | $S_0$       | 0.99                            | 0.26          | 0.20             | 0.23  | 0.23     | 0.02  | 0.02     |
|   |             | $S_3$  | $S_1$    | $S_0$       | 0.15                            | 0.26          | 0.20             | 0.16  | 0.16     | 0.01  | 0.01     |
|   |             |        | $S_2$    | $S_0$       | 0.98                            | 0.13          | 0.20             |       |          |       |          |
|   |             | $S_4$  | $S_2$    | $S_0$       | 0.99                            | 0.13          | 0.20             | 0.17  | 0.17     | 0.01  | 0.01     |
|   |             | $S_5$  | $T_1$    | $T_1$       | 0.98                            | 0.12          | 0.12             | 0.13  | 0.13     | 0.98  | 0.98     |

TABLE S3. Properties of low-lying dimer eigenstates of substituted butadiene dimer ( $\epsilon = 4.0$ ).  $\langle \Psi | \Phi \rangle$  are projections of the dimer state on the direct product of the monomer states  $|\Phi\rangle$ , in the PPP model. The state  $|\Phi\rangle$  is a simple direct product of the states when the states on the two monomers are the same. For two different monomer states,  $|\phi\rangle$  and  $|\chi\rangle$ ,  $|\Phi\rangle = \frac{1}{\sqrt{2}}(|\phi\rangle_I \otimes |\chi\rangle_{II} + |\chi\rangle_I \otimes |\phi\rangle_{II})$ .  $d_I$  and  $d_{II}$  are average double occupancy per site within monomer I and II while  $s_I$  and  $s_{II}$  are the spin value of corresponding monomer units calculated from the spin-spin correlation functions.  $d_{I/II}^{(iso)}$  are the average double occupancies of isolated monomer eigenstates.  $\phi$ -s and  $\Psi$  are the eigenstates of the monomer and the dimer respectively.

| N | Orientation | $\Psi$   | $\phi_I$ | $\phi_{II}$ | $ \langle \Psi   \Phi \rangle $ | $d_I^{(iso)}$ | $d_{II}^{(iso)}$ | $d_I$ | $d_{II}$ | $s_I$ | $s_{II}$ |
|---|-------------|----------|----------|-------------|---------------------------------|---------------|------------------|-------|----------|-------|----------|
| 4 | V           | $S_0$    | $S_0$    | $S_0$       | 0.99                            | 0.26          | 0.26             | 0.27  | 0.27     | 0.01  | 0.01     |
|   |             | $S_1$    | $S_0$    | $S_0$       | 0.10                            | 0.26          | 0.26             | 0.24  | 0.24     | 0.13  | 0.13     |
|   |             |          | $S_1$    | $S_0$       | 0.90                            | 0.23          | 0.26             |       |          |       |          |
|   |             |          | $T_1$    | $T_1$       | 0.14                            | 0.16          | 0.16             |       |          |       |          |
|   |             | $S_2$    | $S_1$    | $S_0$       | 0.98                            | 0.23          | 0.26             | 0.25  | 0.25     | 0.02  | 0.02     |
|   |             | $S_4$    | $S_1$    | $S_0$       | 0.23                            | 0.23          | 0.26             | 0.23  | 0.23     | 0.35  | 0.35     |
|   |             |          | $S_2$    | $S_0$       | 0.75                            | 0.17          | 0.26             |       |          |       |          |
|   |             |          | $T_1$    | $T_1$       | 0.40                            | 0.16          | 0.16             |       |          |       |          |
|   |             | $S_5$    | $S_2$    | $S_0$       | 0.93                            | 0.17          | 0.26             | 0.23  | 0.23     | 0.06  | 0.06     |
|   |             | $S_6$    | $S_1$    | $S_0$       | 0.17                            | 0.23          | 0.26             | 0.23  | 0.23     | 0.44  | 0.44     |
|   |             |          | $S_2$    | $S_0$       | 0.52                            | 0.17          | 0.26             |       |          |       |          |
|   |             |          | $T_1$    | $T_1$       | 0.52                            | 0.16          | 0.16             |       |          |       |          |
|   |             | $S_7$    | $S_1$    | $S_0$       | 0.17                            | 0.23          | 0.26             | 0.25  | 0.25     | 0.32  | 0.32     |
|   |             |          | $S_2$    | $S_0$       | 0.28                            | 0.17          | 0.26             |       |          |       |          |
|   |             |          | $T_1$    | $T_1$       | 0.43                            | 0.16          | 0.16             |       |          |       |          |
|   |             | $S_9$    | $S_2$    | $S_0$       | 0.24                            | 0.17          | 0.26             | 0.21  | 0.21     | 0.45  | 0.45     |
|   |             |          | $T_1$    | $T_1$       | 0.32                            | 0.16          | 0.16             |       |          |       |          |
|   |             | $S_{11}$ | $S_1$    | $S_0$       | 0.17                            | 0.23          | 0.26             | 0.23  | 0.23     | 0.46  | 0.46     |
|   |             |          | $T_1$    | $T_1$       | 0.41                            | 0.16          | 0.16             |       |          |       |          |
|   | H           | $S_0$    | $S_0$    | $S_0$       | 0.99                            | 0.26          | 0.26             | 0.27  | 0.27     | 0.003 | 0.003    |
|   |             | $S_1$    | $S_1$    | $S_0$       | 0.98                            | 0.23          | 0.26             | 0.25  | 0.25     | 0.02  | 0.02     |
|   |             | $S_2$    | $S_1$    | $S_0$       | 0.99                            | 0.23          | 0.26             | 0.25  | 0.25     | 0.01  | 0.01     |
|   |             | $S_3$    | $S_2$    | $S_0$       | 0.96                            | 0.17          | 0.26             | 0.23  | 0.23     | 0.06  | 0.06     |
|   |             | $S_4$    | $S_2$    | $S_0$       | 0.93                            | 0.17          | 0.26             | 0.24  | 0.24     | 0.05  | 0.05     |
|   |             | $S_7$    | $S_2$    | $S_0$       | 0.21                            | 0.17          | 0.26             | 0.21  | 0.21     | 0.68  | 0.68     |
|   |             |          | $T_1$    | $T_1$       | 0.62                            | 0.16          | 0.16             |       |          |       |          |
|   |             | $S_9$    | $T_1$    | $T_1$       | 0.76                            | 0.16          | 0.16             | 0.19  | 0.19     | 0.81  | 0.81     |

TABLE S4. Properties of low-lying dimer eigenstates of substituted hexatriene dimer ( $\epsilon = 1.0$ ).  $\langle \Psi | \Phi \rangle$  are projections of the dimer state on the direct product of the monomer states  $|\Phi\rangle$ , in the PPP model. The state  $|\Phi\rangle$  is a simple direct product of the states when the states on the two monomers are the same. For two different monomer states,  $|\phi\rangle$  and  $|\chi\rangle$ ,  $|\Phi\rangle = \frac{1}{\sqrt{2}}(|\phi\rangle_I \otimes |\chi\rangle_{II} + |\chi\rangle_I \otimes |\phi\rangle_{II})$ .  $d_I$  and  $d_{II}$  are average double occupancy per site within monomer I and II while  $s_I$  and  $s_{II}$  are the spin value of corresponding monomer units calculated from the spin-spin correlation functions.  $d_{I/II}^{(iso)}$  are the average double occupancies of isolated monomer eigenstates.  $\phi$ -s and  $\Psi$  are the eigenstates of the monomer and the dimer respectively.

| N | Orientation | $\Psi$ | $\phi_I$ | $\phi_{II}$ | $ \langle \Psi   \Phi \rangle $ | $d_I^{(iso)}$ | $d_{II}^{(iso)}$ | $d_I$ | $d_{II}$ | $s_I$ | $s_{II}$ |
|---|-------------|--------|----------|-------------|---------------------------------|---------------|------------------|-------|----------|-------|----------|
| 6 | V           | $S_0$  | $S_0$    | $S_0$       | 0.99                            | 0.18          | 0.18             | 0.18  | 0.18     | 0.007 | 0.007    |
|   |             | $S_1$  | $S_1$    | $S_0$       | 0.40                            | 0.14          | 0.18             | 0.18  | 0.18     | 0.67  | 0.67     |
|   |             |        | $S_2$    | $S_0$       | 0.38                            | 0.26          | 0.18             |       |          |       |          |
|   |             |        | $T_1$    | $T_1$       | 0.70                            | 0.15          | 0.15             |       |          |       |          |
|   |             | $S_2$  | $S_1$    | $S_0$       | 0.95                            | 0.14          | 0.18             | 0.17  | 0.17     | 0.07  | 0.07     |
|   |             | $S_3$  | $S_1$    | $S_0$       | 0.24                            | 0.14          | 0.18             | 0.20  | 0.20     | 0.35  | 0.35     |
|   |             |        | $S_2$    | $S_0$       | 0.75                            | 0.26          | 0.18             |       |          |       |          |
|   |             |        | $T_1$    | $T_1$       | 0.39                            | 0.15          | 0.15             |       |          |       |          |
|   |             | $S_4$  | $S_1$    | $S_0$       | 0.86                            | 0.14          | 0.18             | 0.16  | 0.16     | 0.37  | 0.37     |
|   |             |        | $T_1$    | $T_1$       | 0.49                            | 0.15          | 0.15             |       |          |       |          |
|   |             | $S_7$  | $S_2$    | $S_0$       | 0.93                            | 0.26          | 0.18             | 0.22  | 0.22     | 0.08  | 0.08     |
|   | H           | $S_0$  | $S_0$    | $S_0$       | 0.99                            | 0.18          | 0.18             | 0.18  | 0.18     | 0.004 | 0.004    |
|   |             | $S_1$  | $S_1$    | $S_0$       | 0.44                            | 0.14          | 0.18             | 0.16  | 0.16     | 0.84  | 0.84     |
|   |             |        | $T_1$    | $T_1$       | 0.87                            | 0.15          | 0.15             |       |          |       |          |
|   |             | $S_2$  | $S_1$    | $S_0$       | 0.99                            | 0.14          | 0.18             | 0.16  | 0.16     | 0.01  | 0.01     |
|   |             | $S_3$  | $S_1$    | $S_0$       | 0.89                            | 0.14          | 0.18             | 0.16  | 0.16     | 0.32  | 0.32     |
|   |             |        | $T_1$    | $T_1$       | 0.46                            | 0.15          | 0.15             |       |          |       |          |
|   |             | $S_4$  | $S_2$    | $S_0$       | 0.95                            | 0.26          | 0.18             | 0.22  | 0.22     | 0.07  | 0.07     |
|   |             |        | $T_1$    | $T_1$       | 0.11                            | 0.15          | 0.15             |       |          |       |          |
|   |             | $S_5$  | $S_2$    | $S_0$       | 0.96                            | 0.26          | 0.18             | 0.22  | 0.22     | 0.05  | 0.05     |

TABLE S5. Properties of low-lying dimer eigenstates of substituted hexatriene dimer ( $\epsilon = 2.0$ ).  $\langle \Psi | \Phi \rangle$  are projections of the dimer state on the direct product of the monomer states  $|\Phi\rangle$ , in the PPP model. The state  $|\Phi\rangle$  is a simple direct product of the states when the states on the two monomers are the same. For two different monomer states,  $|\phi\rangle$  and  $|\chi\rangle$ ,  $|\Phi\rangle = \frac{1}{\sqrt{2}}(|\phi\rangle_I \otimes |\chi\rangle_{II} + |\chi\rangle_I \otimes |\phi\rangle_{II})$ .  $d_I$  and  $d_{II}$  are average double occupancy per site within monomer I and II while  $s_I$  and  $s_{II}$  are the spin value of corresponding monomer units calculated from the spin-spin correlation functions.  $d_{I/II}^{(iso)}$  are the average double occupancies of isolated monomer eigenstates.  $\phi$ -s and  $\Psi$  are the eigenstates of the monomer and the dimer respectively.

| N | Orientation | $\Psi$ | $\phi_I$ | $\phi_{II}$ | $ \langle \Psi   \Phi \rangle $ | $d_I^{(iso)}$ | $d_{II}^{(iso)}$ | $d_I$ | $d_{II}$ | $s_I$ | $s_{II}$ |
|---|-------------|--------|----------|-------------|---------------------------------|---------------|------------------|-------|----------|-------|----------|
| 6 | V           | $S_0$  | $S_0$    | $S_0$       | 0.99                            | 0.19          | 0.19             | 0.19  | 0.19     | 0.008 | 0.008    |
|   |             | $S_1$  | $S_1$    | $S_0$       | 0.32                            | 0.15          | 0.19             | 0.20  | 0.20     | 0.48  | 0.48     |
|   |             |        | $S_2$    | $S_0$       | 0.59                            | 0.26          | 0.19             |       |          |       |          |
|   |             |        | $T_1$    | $T_1$       | 0.50                            | 0.16          | 0.16             |       |          |       |          |
|   |             | $S_2$  | $S_1$    | $S_0$       | 0.31                            | 0.15          | 0.19             | 0.19  | 0.19     | 0.56  | 0.56     |
|   |             |        | $S_2$    | $S_0$       | 0.62                            | 0.26          | 0.19             |       |          |       |          |
|   |             |        | $T_1$    | $T_1$       | 0.62                            | 0.16          | 0.16             |       |          |       |          |
|   |             | $S_3$  | $S_1$    | $S_0$       | 0.92                            | 0.15          | 0.19             | 0.18  | 0.18     | 0.08  | 0.08     |
|   |             |        | $S_2$    | $S_0$       | 0.17                            | 0.26          | 0.19             |       |          |       |          |
|   |             | $S_4$  | $S_1$    | $S_0$       | 0.85                            | 0.15          | 0.19             | 0.17  | 0.17     | 0.37  | 0.37     |
|   |             |        | $T_1$    | $T_1$       | 0.49                            | 0.16          | 0.16             |       |          |       |          |
|   |             | $S_5$  | $S_1$    | $S_0$       | 0.18                            | 0.15          | 0.19             | 0.22  | 0.22     | 0.08  | 0.08     |
|   |             |        | $S_2$    | $S_0$       | 0.91                            | 0.26          | 0.19             |       |          |       |          |
|   | H           | $S_0$  | $S_0$    | $S_0$       | 0.99                            | 0.19          | 0.19             | 0.20  | 0.20     | 0.004 | 0.004    |
|   |             | $S_1$  | $S_1$    | $S_0$       | 0.25                            | 0.15          | 0.19             | 0.22  | 0.22     | 0.15  | 0.15     |
|   |             |        | $S_2$    | $S_0$       | 0.89                            | 0.26          | 0.19             |       |          |       |          |
|   |             |        | $T_1$    | $T_1$       | 0.24                            | 0.16          | 0.16             |       |          |       |          |
|   |             | $S_2$  | $S_1$    | $S_0$       | 0.31                            | 0.15          | 0.19             | 0.17  | 0.17     | 0.84  | 0.84     |
|   |             |        | $S_2$    | $S_0$       | 0.34                            | 0.26          | 0.19             |       |          |       |          |
|   |             |        | $T_1$    | $T_1$       | 0.87                            | 0.16          | 0.16             |       |          |       |          |
|   |             | $S_3$  | $S_1$    | $S_0$       | 0.99                            | 0.15          | 0.19             | 0.17  | 0.17     | 0.01  | 0.01     |
|   |             | $S_4$  | $S_1$    | $S_0$       | 0.90                            | 0.15          | 0.19             | 0.17  | 0.17     | 0.25  | 0.25     |
|   |             |        | $S_2$    | $S_0$       | 0.16                            | 0.26          | 0.19             |       |          |       |          |
|   |             |        | $T_1$    | $T_1$       | 0.39                            | 0.16          | 0.16             |       |          |       |          |
|   |             | $S_5$  | $S_2$    | $S_0$       | 0.96                            | 0.26          | 0.19             | 0.22  | 0.22     | 0.04  | 0.04     |

TABLE S6. Properties of low-lying dimer eigenstates of substituted hexatriene dimer ( $\epsilon = 4.0$ ).  $\langle \Psi | \Phi \rangle$  are projections of the dimer state on the direct product of the monomer states  $|\Phi\rangle$ , in the PPP model. The state  $|\Phi\rangle$  is a simple direct product of the states when the states on the two monomers are the same. For two different monomer states,  $|\phi\rangle$  and  $|\chi\rangle$ ,  $|\Phi\rangle = \frac{1}{\sqrt{2}}(|\phi\rangle_I \otimes |\chi\rangle_{II} + |\chi\rangle_I \otimes |\phi\rangle_{II})$ .  $d_I$  and  $d_{II}$  are average double occupancy per site within monomer I and II while  $s_I$  and  $s_{II}$  are the spin value of corresponding monomer units calculated from the spin-spin correlation functions.  $d_{I/II}^{(iso)}$  are the average double occupancies of isolated monomer eigenstates.  $\phi$ -s and  $\Psi$  are the eigenstates of the monomer and the dimer respectively.

| N | Orientation | $\Psi$ | $\phi_I$ | $\phi_{II}$ | $ \langle \Psi   \Phi \rangle $ | $d_I^{(iso)}$ | $d_{II}^{(iso)}$ | $d_I$ | $d_{II}$ | $s_I$ | $s_{II}$ |
|---|-------------|--------|----------|-------------|---------------------------------|---------------|------------------|-------|----------|-------|----------|
| 6 | V           | $S_0$  | $S_0$    | $S_0$       | 0.98                            | 0.24          | 0.24             | 0.24  | 0.24     | 0.017 | 0.017    |
|   |             | $S_1$  | $S_0$    | $S_0$       | 0.12                            | 0.24          | 0.24             | 0.23  | 0.23     | 0.25  | 0.25     |
|   |             |        | $S_1$    | $S_0$       | 0.81                            | 0.25          | 0.24             |       |          |       |          |
|   |             |        | $T_1$    | $T_1$       | 0.26                            | 0.20          | 0.20             |       |          |       |          |
|   |             | $S_2$  | $S_1$    | $S_0$       | 0.95                            | 0.25          | 0.24             | 0.24  | 0.24     | 0.05  | 0.05     |
|   |             | $S_3$  | $S_1$    | $S_0$       | 0.45                            | 0.25          | 0.24             | 0.22  | 0.22     | 0.66  | 0.66     |
|   |             |        | $S_2$    | $S_0$       | 0.40                            | 0.19          | 0.24             |       |          |       |          |
|   |             |        | $T_1$    | $T_1$       | 0.70                            | 0.20          | 0.20             |       |          |       |          |
|   |             | $S_4$  | $S_1$    | $S_0$       | 0.15                            | 0.25          | 0.24             | 0.23  | 0.23     | 0.36  | 0.36     |
|   |             |        | $S_2$    | $S_0$       | 0.17                            | 0.19          | 0.24             |       |          |       |          |
|   |             |        | $T_1$    | $T_1$       | 0.49                            | 0.20          | 0.20             |       |          |       |          |
|   |             | $S_5$  | $S_1$    | $S_0$       | 0.15                            | 0.25          | 0.24             | 0.22  | 0.22     | 0.08  | 0.08     |
|   |             |        | $S_2$    | $S_0$       | 0.92                            | 0.19          | 0.24             |       |          |       |          |
|   |             | $S_6$  | $S_2$    | $S_0$       | 0.78                            | 0.19          | 0.24             | 0.22  | 0.22     | 0.44  | 0.44     |
|   |             |        | $T_1$    | $T_1$       | 0.53                            | 0.20          | 0.20             |       |          |       |          |
|   | H           | $S_0$  | $S_0$    | $S_0$       | 0.99                            | 0.24          | 0.24             | 0.24  | 0.24     | 0.004 | 0.004    |
|   |             | $S_1$  | $S_1$    | $S_0$       | 0.96                            | 0.25          | 0.24             | 0.24  | 0.24     | 0.03  | 0.03     |
|   |             | $S_2$  | $S_1$    | $S_0$       | 0.99                            | 0.25          | 0.24             | 0.24  | 0.24     | 0.02  | 0.02     |
|   |             | $S_3$  | $S_2$    | $S_0$       | 0.30                            | 0.19          | 0.24             | 0.21  | 0.21     | 0.85  | 0.85     |
|   |             |        | $T_1$    | $T_1$       | 0.84                            | 0.20          | 0.20             |       |          |       |          |
|   |             | $S_4$  | $S_2$    | $S_0$       | 0.88                            | 0.19          | 0.24             | 0.22  | 0.22     | 0.30  | 0.30     |
|   |             |        | $T_1$    | $T_1$       | 0.41                            | 0.20          | 0.20             |       |          |       |          |
|   |             | $S_5$  | $S_2$    | $S_0$       | 0.88                            | 0.19          | 0.24             | 0.22  | 0.22     | 0.14  | 0.14     |



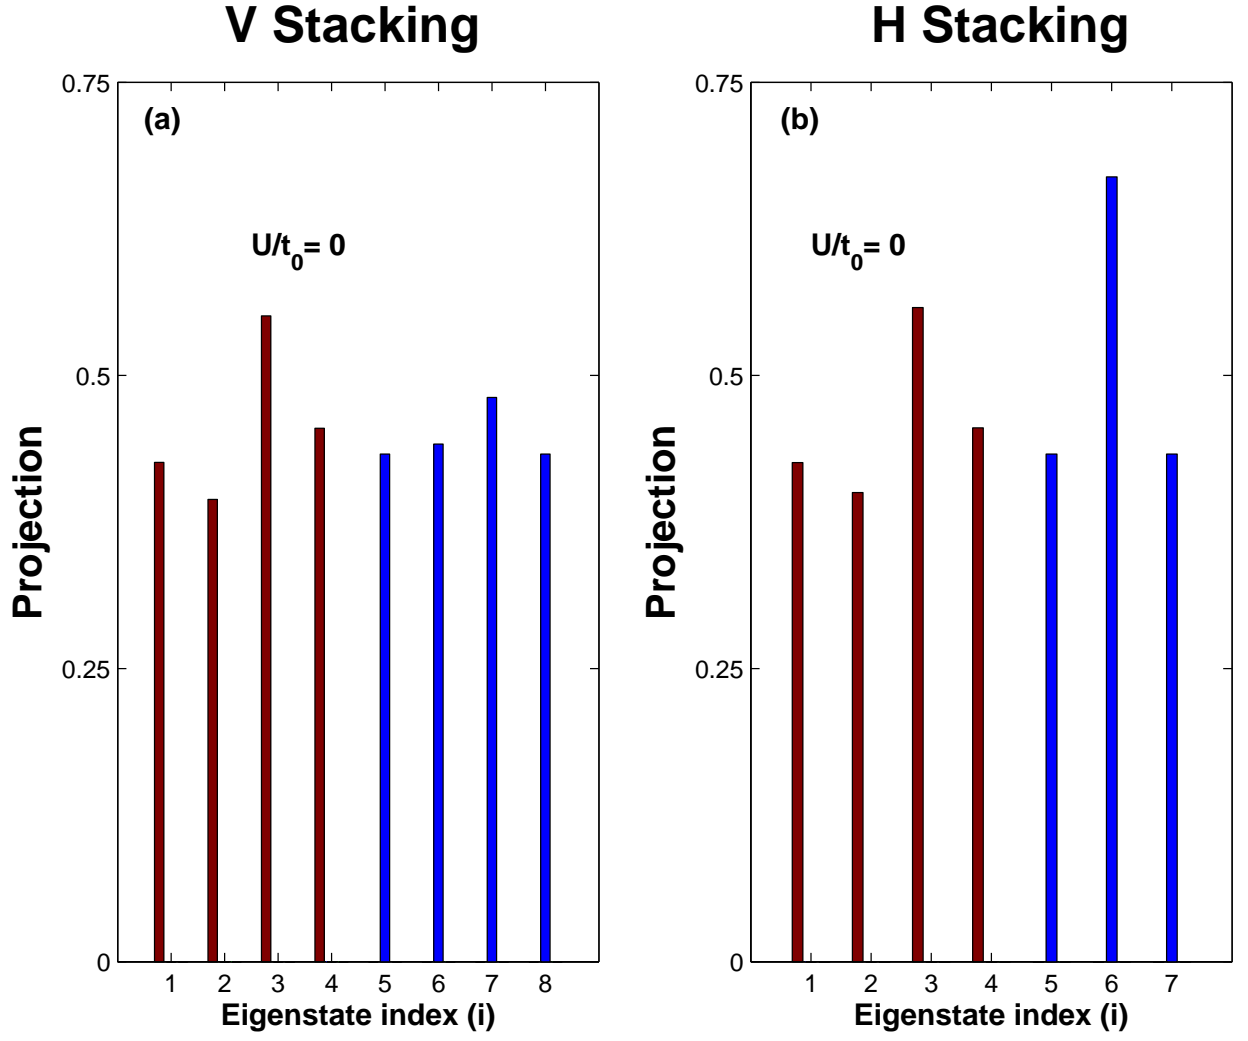

FIG. S1. (Color online) Indexing of the many-body eigenstates of the full system Hamiltonian with significant overlaps with  $1^1B \otimes 1^1A$  (dark brown) and  $T_1 \otimes T_1$  (dark blue). The stacking type is indicated by the letters V and H in both subfigures. Note that no eigenstates of  $H_{full}$  has significant overlap with both  $1^1B \otimes 1^1A$  and  $T_1 \otimes T_1$  simultaneously.

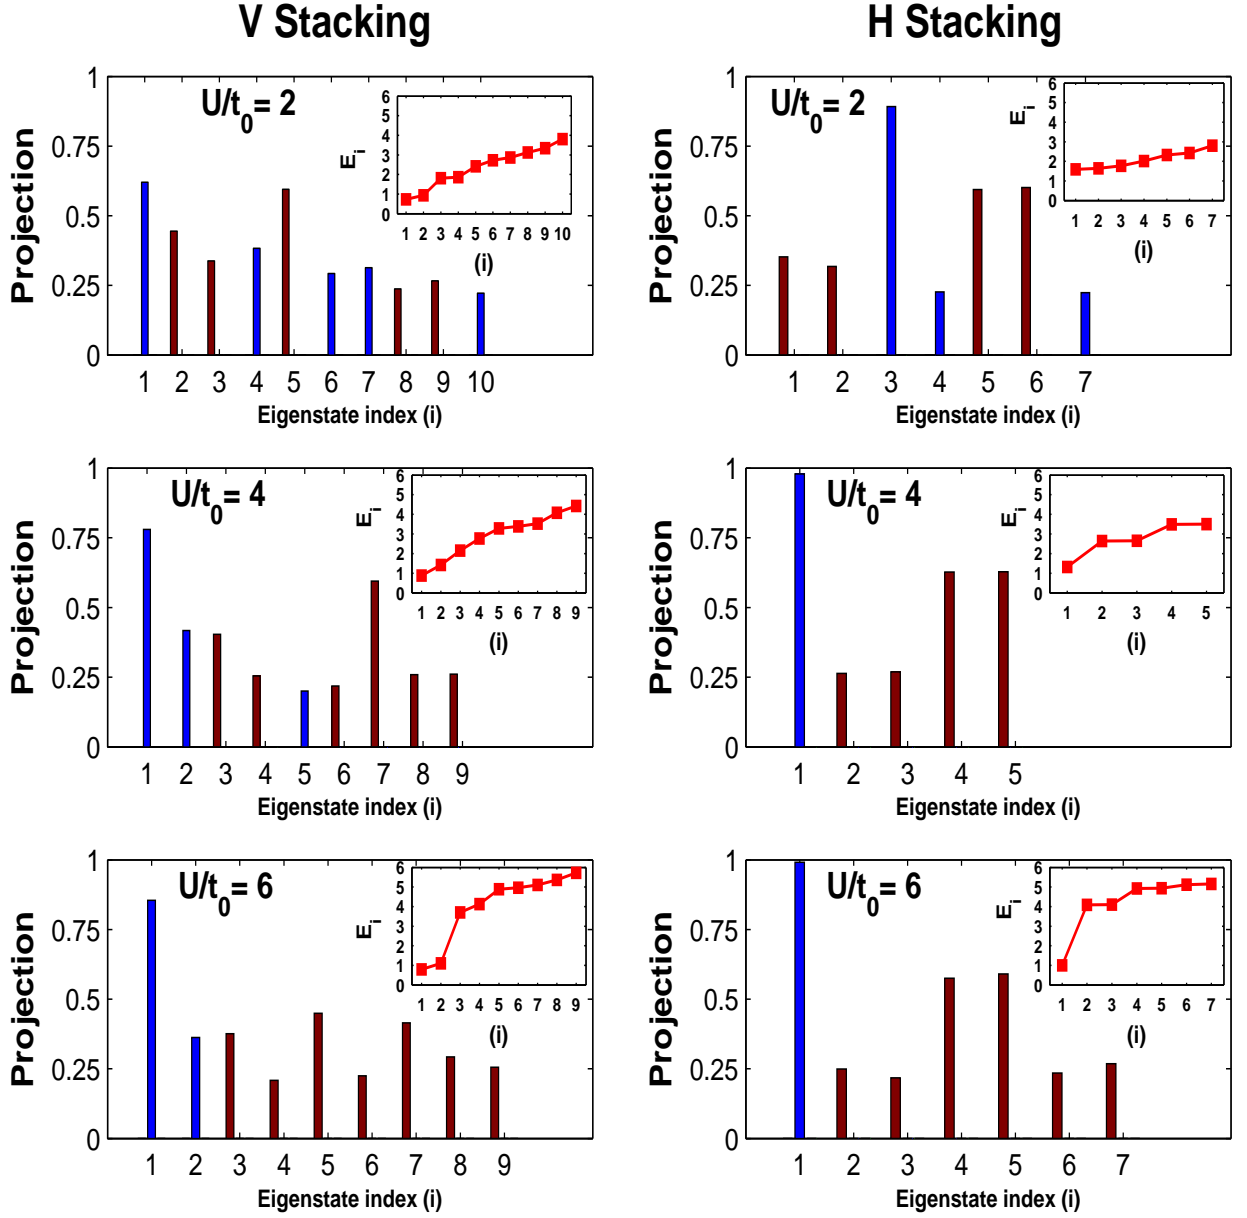

FIG. S2. (Color online) Significant projections of  $1^1B \otimes 1^1A$  and  $T_1 \otimes T_1$  with eigenstates of the dimer system within Hubbard model are shown as histograms. The left panel corresponds to V stacking while the right panel corresponds to H stacking. The color indices are as follows: dark brown, projection to initial state,  $P_i \equiv \langle 1^1B \otimes 1^1A | \psi_i \rangle$ ; dark blue, projection to final state,  $P_f \equiv \langle T_1 \otimes T_1 | \psi_i \rangle$ ; dark green,  $P_i \times P_f$ . Inset:  $E_i$ , the energy of the significant eigenstate 'i' as measured from the ground state of the full system is shown.

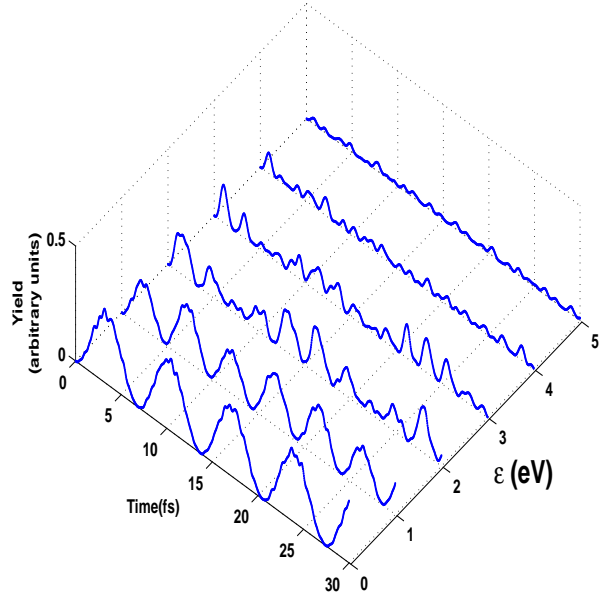

(A)

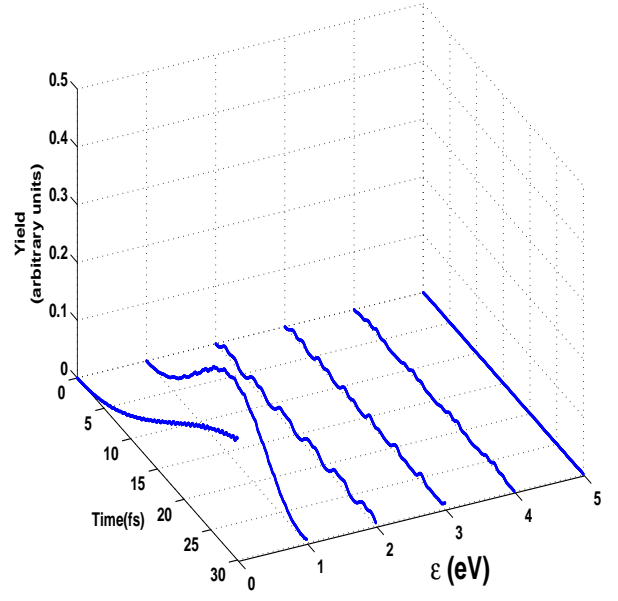

(B)

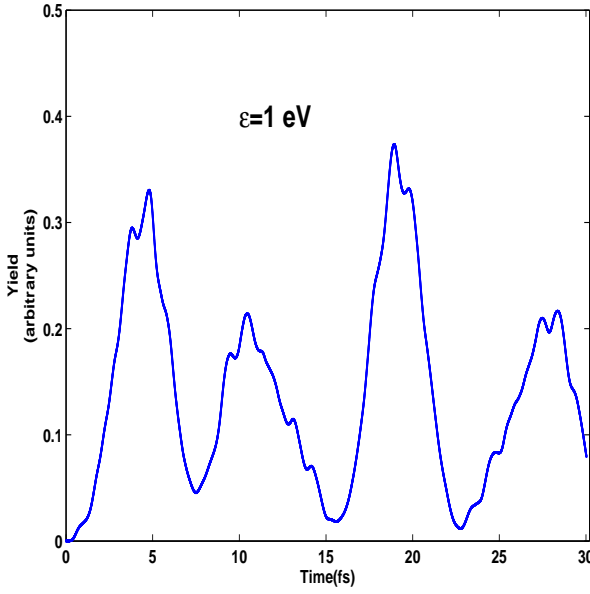

(C)

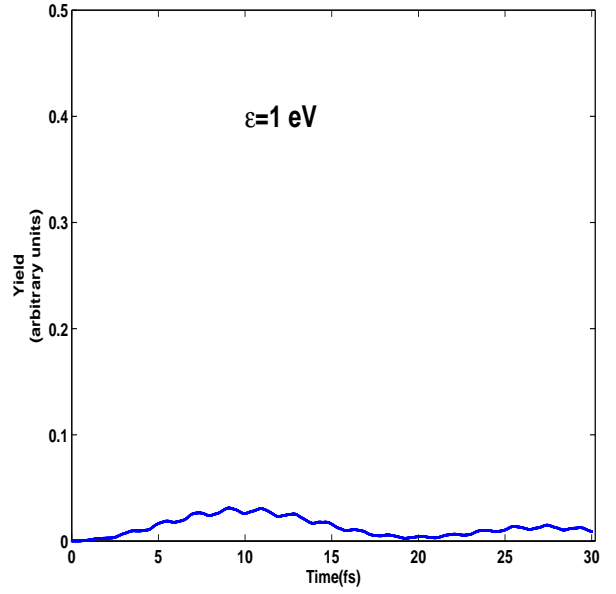

(D)

FIG. S3. (Color online) Yield as a function of time and donor-acceptor strength  $\epsilon$  for singlet fission in 1,3-butadiene dimer from the lowest singlet excited state  $S_1$  in (A) V stacking and (B) H stacking. For  $\epsilon = 1$  eV, the yield from the optical singlet state is also shown in (C) V stacking and (D) H stacking. For  $\epsilon \geq 2$  eV, we find that the lowest excited state is also the state with large transition dipole moment.

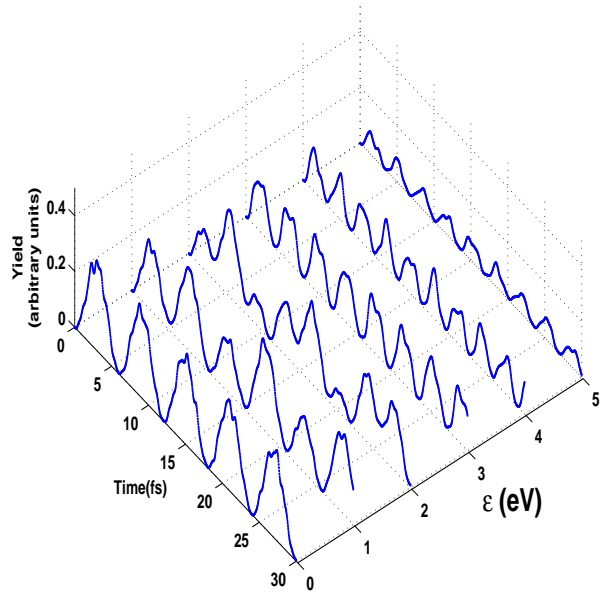

(A)

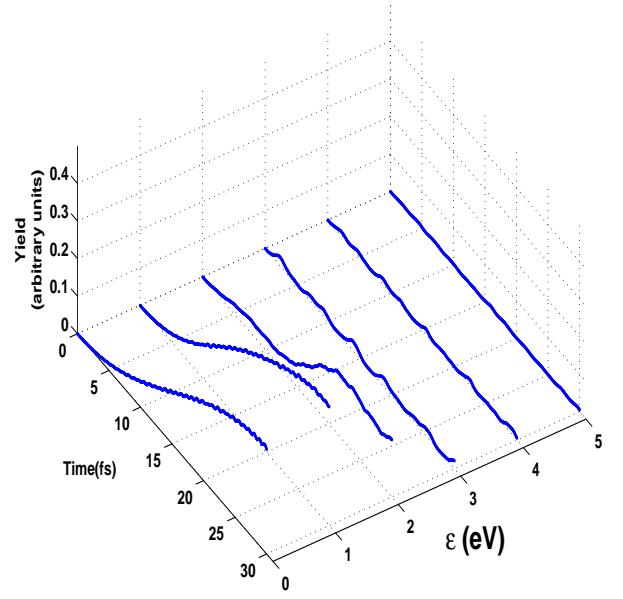

(B)

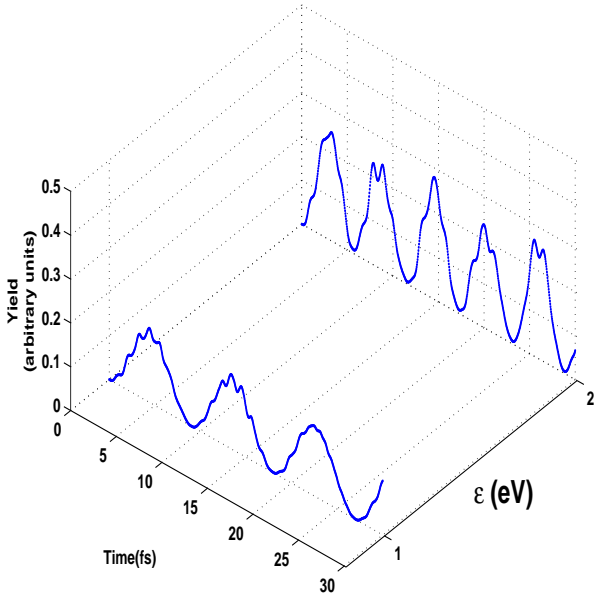

(C)

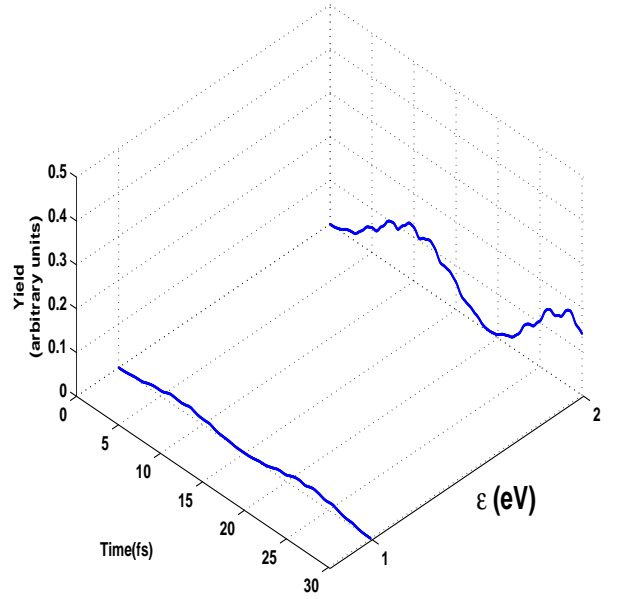

(D)

FIG. S4. (Color online) Yield as a function of time and donor-acceptor strength  $\epsilon$  for singlet fission in 1,3,5-hexatriene dimer from the lowest singlet excited state  $S_1$  in (A) V stacking and (B) H stacking. For  $\epsilon = 1$  eV and 2 eV, the yield from the optical singlet state is also shown in (C) V stacking and (D) H stacking. For  $\epsilon \geq 3$  eV, we find that the lowest excited state is also the state with large transition dipole moment.

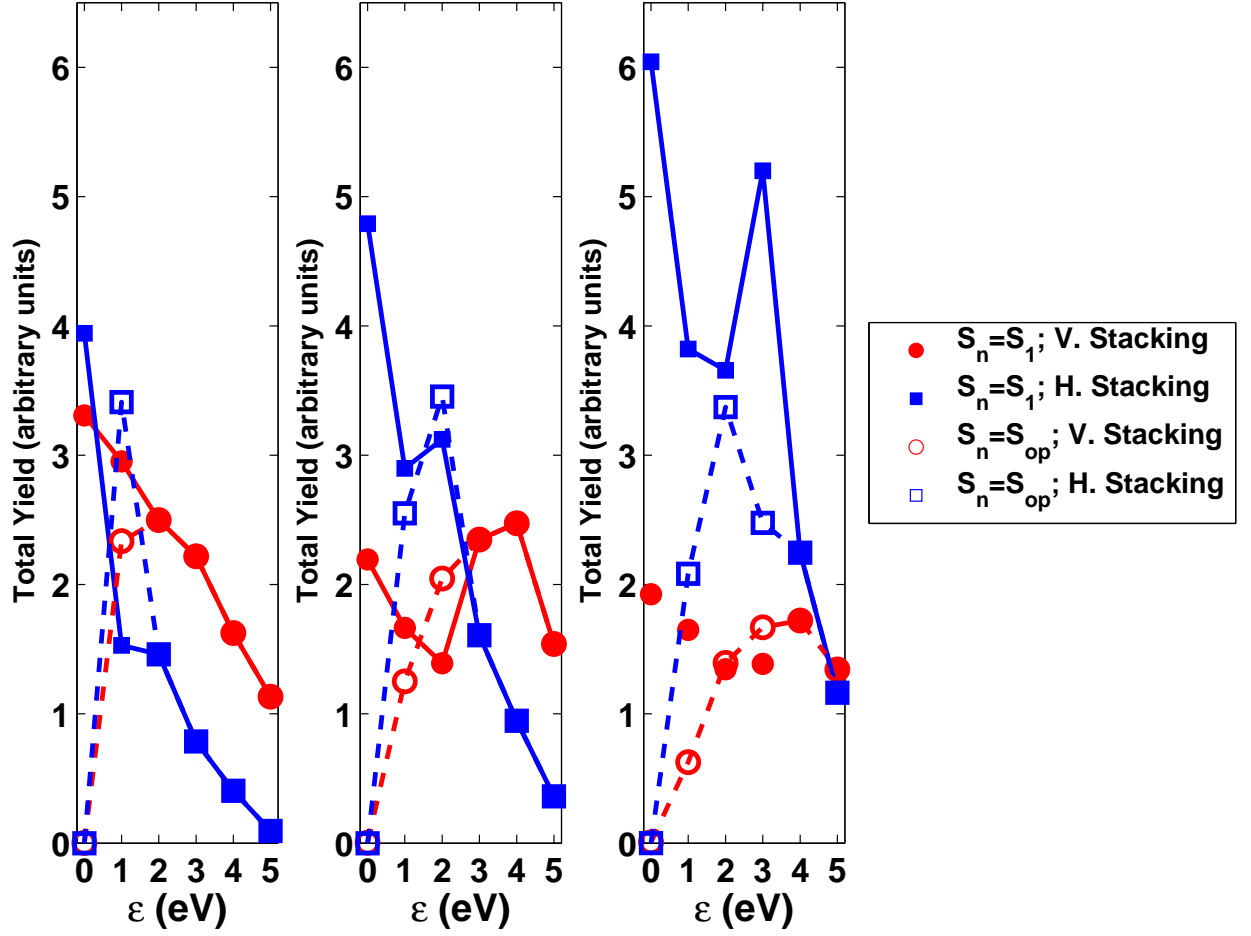

FIG. S5. (Color online) Total yield in unsubstituted and substituted polyene dimers are plotted as a function of substitution strength  $\epsilon$  for both vertical and horizontal stacking orientations within the PPP model. The left, center and right panels correspond to monomers of 4, 6 and 8 sites. The color and symbol indices are given in the following and same in all three panels: red filled circle,  $S_n \equiv S_1$ , V stacking; blue filled square,  $S_n \equiv S_1$ , H stacking. The open symbols represent  $S_n \equiv S_{op}$  scenarios in the corresponding systems. Beyond a certain  $\epsilon$ ,  $S_n \equiv S_1 \equiv S_{op}$  and the curves coincide. The solid and broken lines are given only as a guide to the eyes. Here  $|t_\perp| = X_\perp = 0.5$  eV.

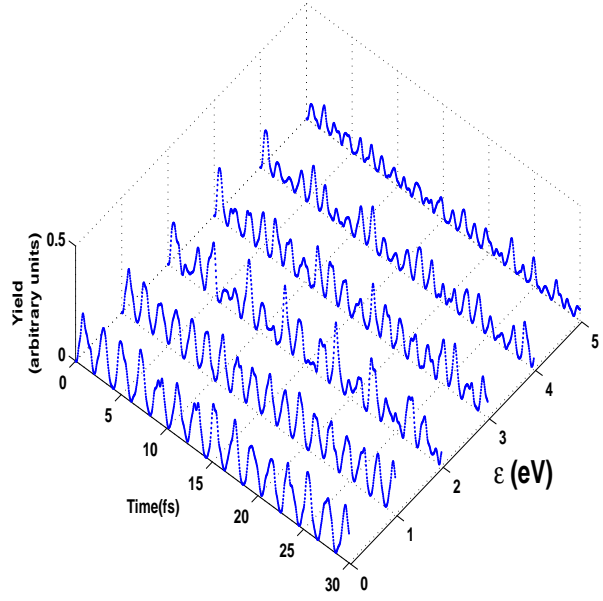

(A)

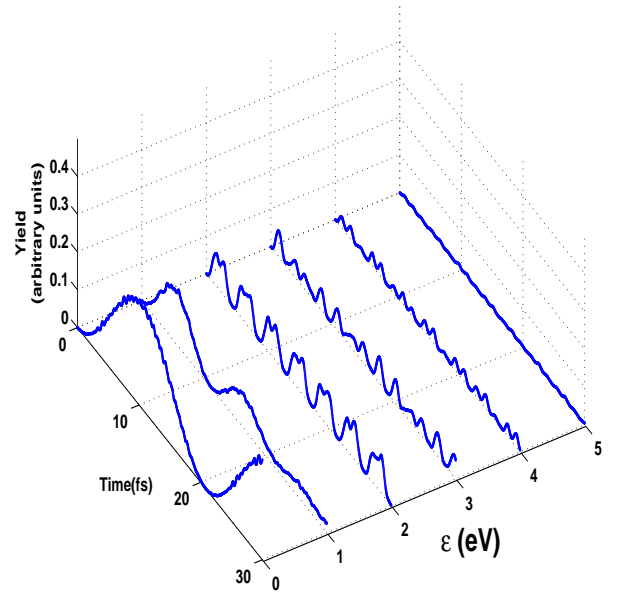

(B)

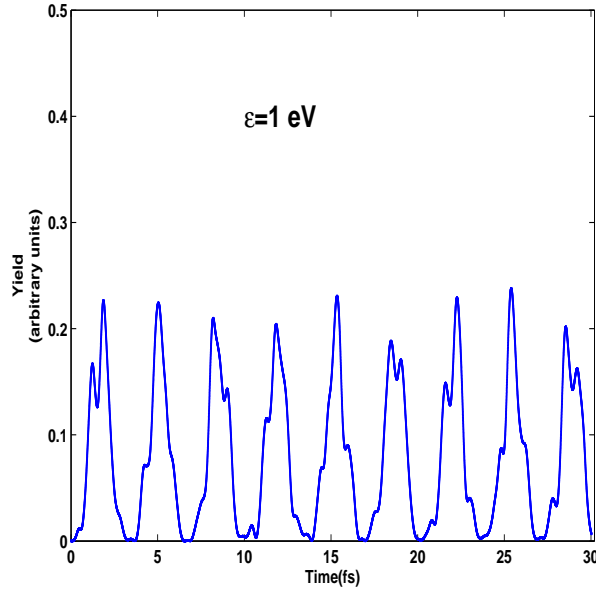

(C)

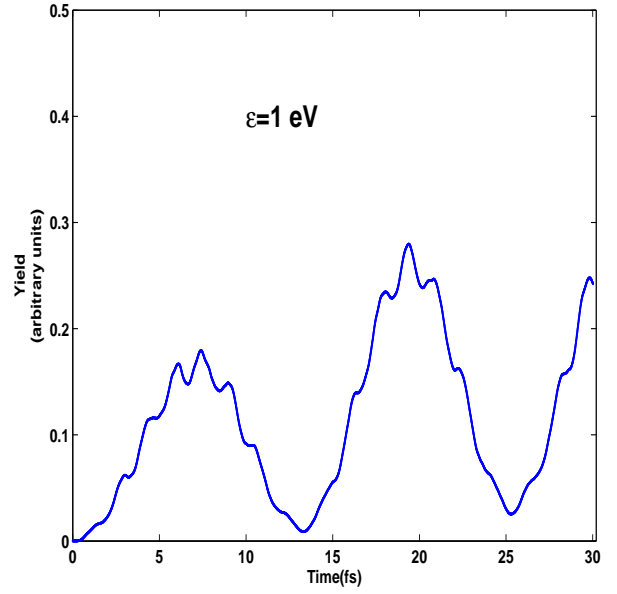

(D)

FIG. S6. (Color online) Yield as a function of time and donor-acceptor strength  $\epsilon$  for singlet fission in 1,3-butadiene dimer from the lowest singlet excited state  $S_1$  in (A) V stacking and (B) H stacking. For  $\epsilon = 1$  eV, the yield from the optical singlet state is also shown in (C) V stacking and (D) H stacking. For  $\epsilon \geq 2$  eV, we find that the lowest excited state is also the state with large transition dipole moment. Here  $|t_\perp| = X_\perp = 0.5$  eV.

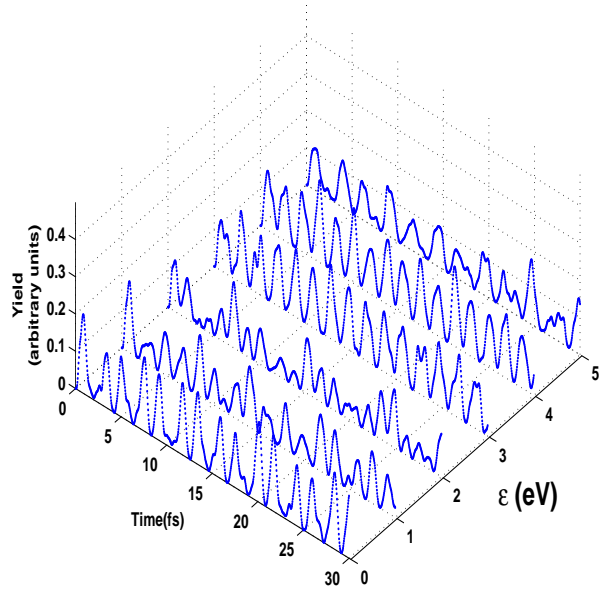

(A)

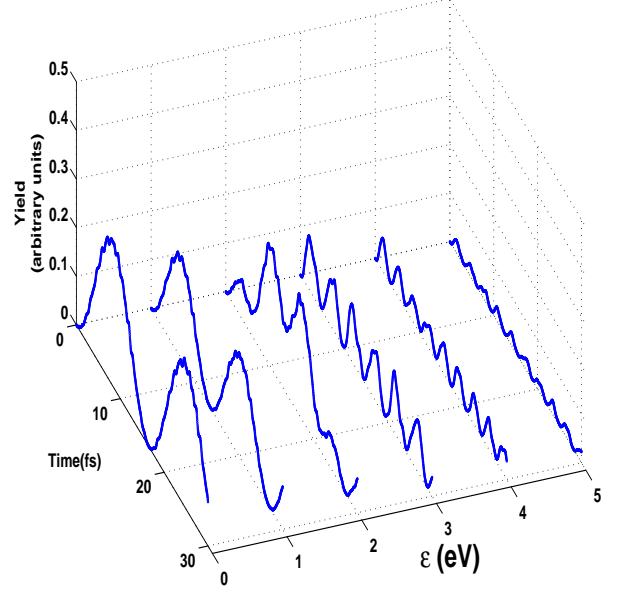

(B)

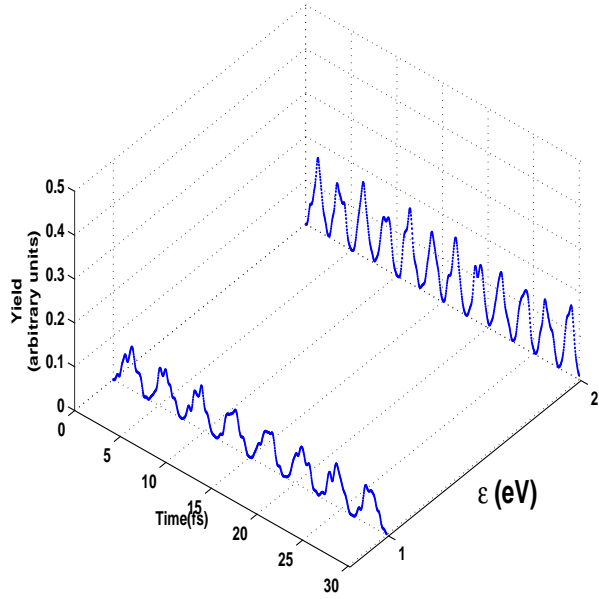

(C)

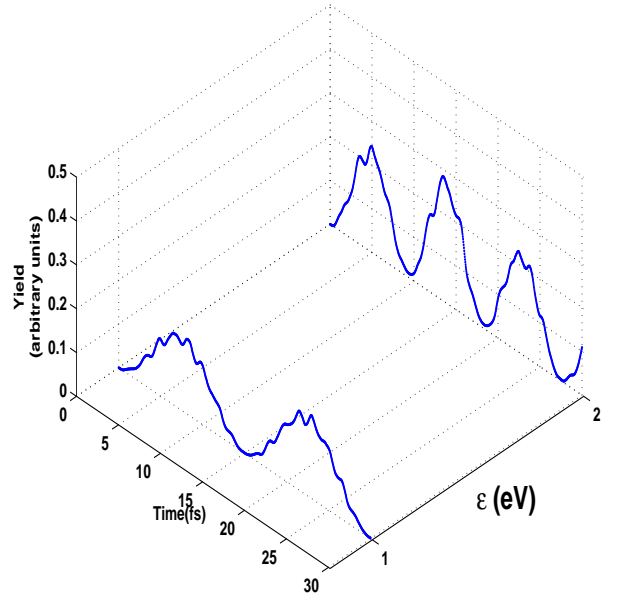

(D)

FIG. S7. (Color online) Yield as a function of time and donor-acceptor strength  $\epsilon$  for singlet fission in 1,3,5-hexatriene dimer from the lowest singlet excited state  $S_1$  in (A) V stacking and (B) H stacking. For  $\epsilon = 1$  eV and 2 eV, the yield from the optical singlet state is also shown in (C) V stacking and (D) H stacking. For  $\epsilon \geq 3$  eV, we find that the lowest excited state is also the state with large transition dipole moment. Here  $|t_\perp| = X_\perp = 0.5$  eV.

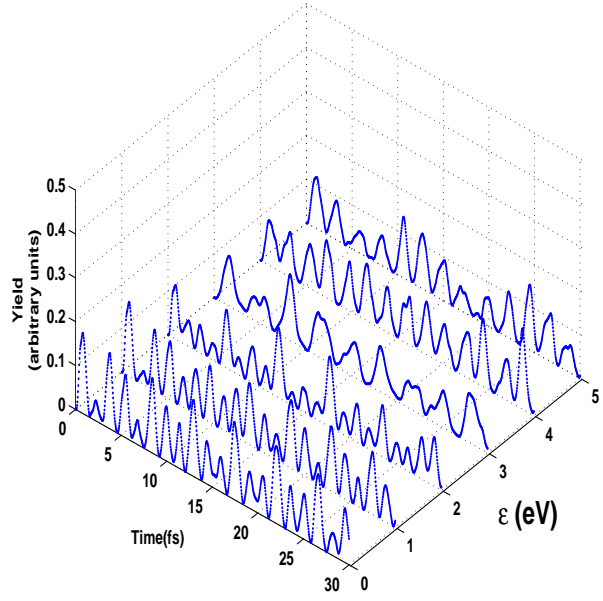

(A)

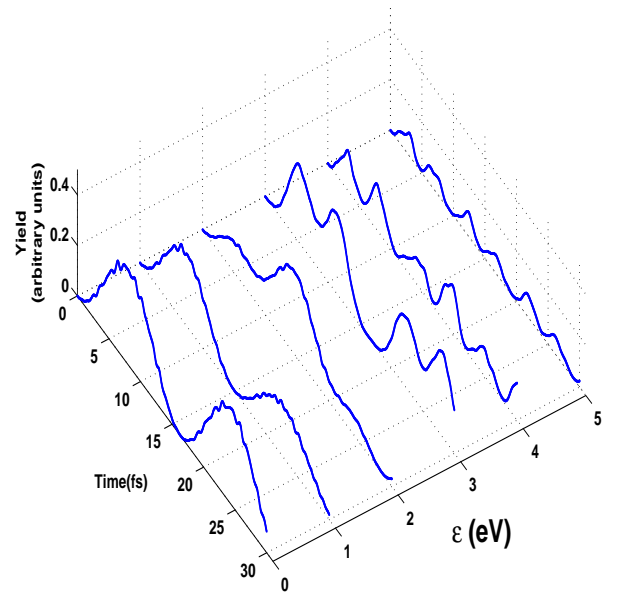

(B)

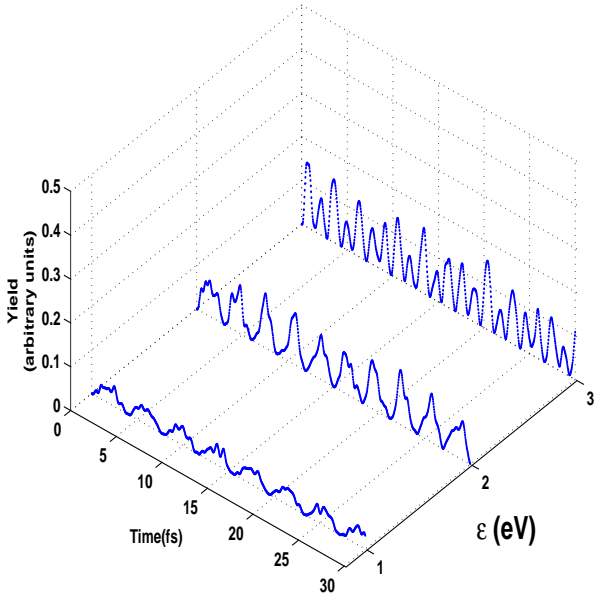

(C)

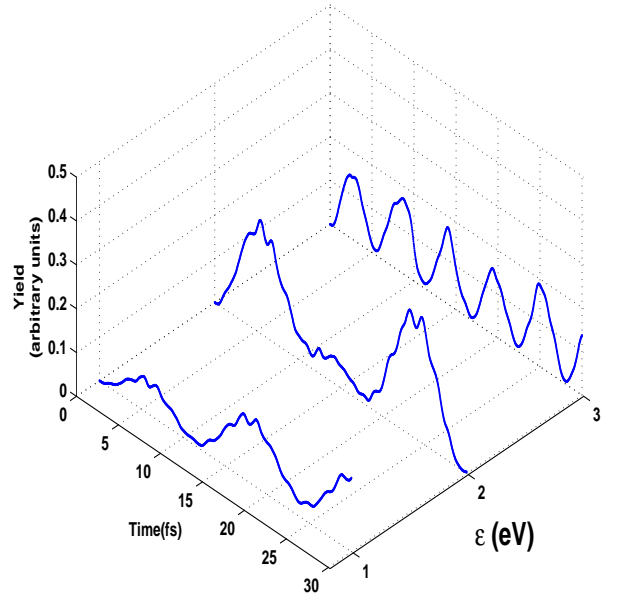

(D)

FIG. S8. (Color online) Yield as a function of time and donor-acceptor strength  $\epsilon$  for singlet fission in 1,3,5,7-octatetraene dimer from the lowest singlet excited state  $S_1$  in (A) V stacking and (B) H stacking. For  $\epsilon = 1, 2$  and  $3$  eV, the yield from the optical singlet state is also shown in (C) V stacking and (D) H stacking. For  $\epsilon \geq 4$  eV, we find that the lowest excited state is also the state with large transition dipole moment. Here  $|t_\perp| = X_\perp = 0.5$  eV.
